# Supplementary material for: Training-free Dense-Aligned Diffusion Guidance for Modular Conditional Image Synthesis
Source: arXiv:2504.01515 source file (2025-04-03)
Supplement: Supplementary file 1 [file X_suppl.tex]

\clearpage
\setcounter{page}{1}
\maketitlesupplementary

In this supplementary material, we provide additional information in the following three aspects:

\textbf{A.} discussion on synthesis with depth map and text;

\textbf{B.} quantitative analysis of synthesis with bounding box and text;

\textbf{C.} additional visualizations on various baselines.

\section{Image Synthesis Results with Depth Map and Text}
\label{sec:rationale}
We evaluate performance based on descriptions and depth maps using ImageNet-R-TI2I dataset \cite{tumanyan2023plug} as our benchmark. This dataset consists of 30 images across 10 object categories. Original images are converted into corresponding depth maps following the pipeline outlined in \cite{zhang2023adding}. To quantify the accuracy of image synthesis, we employ Root Mean Squared Error (RMSE), which measures the pixel-wise discrepancy between the synthesized and original images. Since the given conditions specify a single foreground object, we utilize only the $\mathcal{L}_{cvg}$ component in the DGA module to optimize alignment and fidelity.

\begin{figure}[htb]
    \centering
    \includegraphics[width=0.47\textwidth]{sec/FIG/suppl_depth.jpg} 
    \caption{
    Visualization comparison between our approach (ControlNet \cite{zhang2023adding} + DGA) and other baselines, under varying descriptions and depth maps. Our approach demonstrates a superior ability to adhere to the positional information within the depth map.
    }
    \label{FIG5_1}
\end{figure}

We use ControNet \cite{zhang2023adding} as a baseline model to evaluate the effectiveness of our DGA module in aligning spatial configurations represented by depth maps. Tab.~\ref{TABLE_2} summarized the RMSE score on ImageNet-R-TI2I dataset \cite{tumanyan2023plug}. Our DGA module improves the performance over ControlNet by approximately 4.73\%. This substantial gain is because our $\mathcal{L}_{cvg}$ component enhances the overlap between the object’s layout and its depth map. Fig.~\ref{FIG5_1} reveals a clear and consistent conclusion.  

\begin{table}[htbp]
\centering
\caption{Quantitative comparison under the textual description and depth map conditions. The data are derived from the ImageNet-R-TI2I dataset \cite{tumanyan2023plug}. The evaluation metric used is RMSE. Since the conditions specify only one foreground object, we utilize the $\mathcal{L}_{cvg}$ component in the DGA module. The best results are \textbf{highlighted}.}
\label{TABLE_2}
\begin{tabular}{cccc}
\toprule[1.5pt]
Methods  & Venue & RMSE $ \downarrow $ \\ % & CLIPScore $ \uparrow $ \\
\midrule
Stable Diffusion \cite{rombach2022high} & CVPR2022 & 92.42 \\ %& 0.1451 \\
\midrule
ControlNet \cite{zhang2023adding} & CVPR2023 & 47.73 \\ %& 0.1372 \\
\rowcolor{gray!10}
+ DGA & - & \textbf{45.47} \\ %& - \\
%\rowcolor{gray!10}
%+ DGA + DCA & - & - \\ %& - \\
\bottomrule[1.5pt]
\end{tabular}
\end{table}
% 

%\section{Limitations}
\section{Additional Quantitative Results}
Additional quantitative results of image synthesis with bounding box and text are shown in Tab.~\ref{TABLE_ADD}. Our DGA and DCA modules are also effective in this scenario.

\begin{table}[h]
\centering
\caption{Quantitative comparison under the textual description and bounding box conditions provided by \cite{saharia2022photorealistic,phung2024grounded}. The evaluation metric used is positional \cite{bakr2023hrs}. The baseline model of our approach is A$\&$R \cite{phung2024grounded}.  The best results are \textbf{highlighted}.}
\label{TABLE_ADD}
\resizebox{\columnwidth}{!}{ 
\begin{tabular}{ccc}
\toprule[1.5pt]
Methods  & Venue & Positional $ \uparrow $ \\
\midrule
Stable Diffusion \cite{rombach2022high} & CVPR2022 & 12.50 \\
Attend-and-Excite \cite{chefer2023attend} & SIGGRAPH2023 & 20.50 \\
DenseDiffusion \cite{kim2023dense} & ICCV2023 & 30.50 \\
BoxDiff \cite{xie2023boxdiff} & ICCV2023 & 32.50 \\
MultiDiffusion \cite{bar2023multidiffusion} & ICML2023 & 36.00 \\
Layout-guidance \cite{chen2024training} & WACV2024 &  36.50 \\
\midrule
A$\&$R \cite{phung2024grounded} & CVPR2024 & 43.50 \\
\rowcolor{gray!10}
+ DGA  & - & 45.00  \\
\rowcolor{gray!10}
+ DGA + DCA & - & \textbf{47.50} \\
\bottomrule[1.5pt]
\end{tabular}
}
\end{table}

\section{Additional Visualization Results}
\label{sec:rationale}
We conduct additional visualization comparison. We use Stable Diffusion v1.5 \cite{rombach2022high} as a baseline model to evaluate the effectiveness of our DCA module in aligning concepts within descriptions. Visualization results are shown in Fig.~\ref{FIG_S2}. We use  Dense Diffusion \cite{kim2023dense} as a baseline model to evaluate the effectiveness of our DGA module in aligning spatial configurations represented by segmentation masks; and our DCA module in aligning geometric concepts within descriptions. Visualization results are shown in Fig.~\ref{FIG_S3}.

As shown in Fig.~\ref{FIG_S2}, our approach accurately generates multiple objects, \textit{e.g.}, two bears (row 1), two people with a parachute (row 2), and a couple with a dog (row 4), demonstrating its superior compositional reasoning capability. Additionally, our model effectively synthesizes small yet important elements, such as the penguin napkin holder (row 3), highlighting its enhanced ability to preserve fine details. Furthermore, the objects in our results exhibit more natural interactions with their environment, \textit{e.g.}, the polar bears engaging with water (row 1) and the parachute partially resting on the sand (row 2), indicating improved spatial and contextual alignment.

\begin{figure}[htbp]
    \centering
    \includegraphics[width=1.0\columnwidth]{sec/FIG/suppl_description.jpg} 
    \caption{Visualization comparison between our approach (Stable Diffusion v1.5 \cite{rombach2022high} + DCA) and its baseline under varying descriptions. Our approach exhibits superior compositional reasoning, detail preservation, and contextual alignment. }
    \label{FIG_S2}
\end{figure}

As shown in Fig.~\ref{FIG_S3}, our approach ensures that multiple objects are correctly positioned relative to each other, \textit{e.g.}, the surfboard is properly placed on the car roof (row 1), and the dog is accurately seated on the bench (row 2), demonstrating its superior object placement capability. Additionally, our generated objects maintain coherent geometry and proportions, \textit{e.g.}, the cat and laptop are well-defined and spatially distinguishable (row 3), highlighting the model’s ability to preserve structural consistency. Furthermore, our method effectively respects depth relationships, \textit{e.g.}, the couch and TV exhibit a realistic depth ordering (row 4), ensuring proper scene composition.

\begin{figure}[htbp]
    \centering
    \includegraphics[width=1.0\columnwidth]{sec/FIG/suppl_mask.jpg} 
    \caption{Visualization comparison between our approach (Dense Diffusion \cite{kim2023dense} + DGA+ DCA) and its baseline, under varying descriptions and segmentation masks.. Our approach can satisfy both conditions.}
    \label{FIG_S3}
\end{figure}
